# Supplementary material for: Evaluating Disentanglement in Generative Models Without Knowledge of Latent Factors
Source: arXiv:2210.01760 source file (2022-10-04)
Supplement: Supplementary file 1 [file appendix.tex]

\section{Appendix}
\begin{table}[]
\caption{Encoder and Decoder implementation details.}
\label{tab:arch}
\begin{center}
\begin{tabular}{l}
\hline
Encoder           \\
\hline 
Input: $64 \times 64\times \text{number of channels}$ \\
$4\times 4$ conv, $32$ ReLU, stride $2$ \\
$4\times 4$ conv, $32$ ReLU, stride $2$ \\
$4\times 4$ conv, $64$ ReLU, stride $2$ \\
$4\times 4$ conv, $64$ ReLU, stride $2$ \\
FC $256$, F$2$ $2\times 10$ \\
\hline
Decoder \\
\hline
$4\times 4$ deconv, number of channels, stride $2$ \\
Input: $\mathbb{R}^d$ \\
FC, $256$ ReLU \\
FC, $4\times 4\times 64$ ReLU \\
FC, $4\times 4$ conv, $64$ ReLU, stride $2$ \\
FC, $4\times 4$ conv, $32$ ReLU, stride $2$ \\
$4\times 4$ deconv, $32$ ReLU, stride $2$\\ \hline
\end{tabular}
\end{center}
\end{table}
\begin{table}[h]
\caption{Common hyperparameters}
\label{tab:hyperparam}
\begin{center}
\begin{tabular}{ll}
\hline
Parameter          & Values          \\
\hline 
Batch size & $[32, 64, 128, 256]$ \\
Latent space dimension & $[2, 4, 8, 16, 32]$ \\
Optimizer & SGD \\
Learning rate & $[0.1, 0.01, 0.001]$ \\
Momentum coefficient & $0.9$ \\
Decoder & Bernoulli \\
Weight initialization & Glorot Normal for $W$s, Normal for $b$s  \\
Random seed & $[0,1,2,3,4]$
\end{tabular}
\end{center}
\end{table}
